# Supplementary material for: Classical Density Functional Theory applied to the solid state
Source: arXiv:2009.14586 source file (2020-09-30)
Supplement: Supplementary file 1 [file SupplementaryMaterial.pdf]

# Supplementary Material for "Classical Density Functional Theory applied to the solid state"

James F. Lutsko* and Cédric Schoonen
*Center for Nonlinear Phenomena and Complex Systems CP 231,*
*Université Libre de Bruxelles, Blvd. du Triomphe, 1050 Brussels, Belgium*
(Dated: September 30, 2020)

## I. INTRODUCTION

This document consists of three sections. The first gives our derivation of closed analytic formulae for implementing the FMT weight functions in real space based on trilinear interpolation of the density field on a Cartesian lattice. This is followed by a second Section giving some numerical benchmarks for our calculations to give some idea of the sensitivity of our results the lattice spacing. In the final Section we give information concerning our implementation of the FIRE algorithm.

## II. THE FMT WEIGHTS

### A. General form

The calculation is performed using a rectangular lattice with lattice spacings $\Delta_a$ with $a = x, y, z$ and lattice sites $\mathbf{R}_{\mathbf{I}}$ where the superindex is $\mathbf{I} \equiv (I_x, I_y, I_z)$. For any given position $\mathbf{r}$ we denote as $\mathbf{I}(\mathbf{r})$ the index of the lattice site $\mathbf{R}_{\mathbf{I}(\mathbf{r})}$ which is the corner of the of the computational cell containing the point $\mathbf{r}$ which satisfies $R_{\mathbf{I}_a(\mathbf{r})} \leq r_a < R_{I_a(\mathbf{r})} + \Delta_a$ . The density is approximated using trilinear interpolation,

$$\begin{aligned}\rho(\mathbf{r}) &= \sum_{J_x=0,1}\sum_{J_y=0,1}\sum_{J_z=0,1} A_{\mathbf{J}}\left(\mathbf{r}-\mathbf{R}_{\mathbf{I}(\mathbf{r})}\right)\rho_{\mathbf{I}(\mathbf{r})+\mathbf{J}} \\ &\equiv \sum_{\mathbf{J}=0,1} A_{\mathbf{J}}\left(\mathbf{r}-\mathbf{R}_{\mathbf{I}(\mathbf{r})}\right)\rho_{\mathbf{I}(\mathbf{r})+\mathbf{J}}\end{aligned} \tag{1}$$

where the second line introduces a short-hand notation and where the matrix $A_{\mathbf{J}}(\mathbf{r})$ is

$$A_{\mathbf{J}}(\mathbf{r}) = \prod_{a=x,y,z}\left(\frac{\Delta_a - r_a}{\Delta_a}\delta_{J_a=0} + \frac{r_a}{\Delta_a}\delta_{J_a=1}\right). \tag{2}$$

Inserting the trilinear interpolant into the definition of the fundamental measures at lattice site $\mathbf{R}_s$ gives

$$n_{\mathbf{S}}^{(\alpha)} \equiv n^{(\alpha)}(\mathbf{R}_{\mathbf{S}}) = \int w^{(\alpha)}(\mathbf{R}_{\mathbf{S}}-\mathbf{r})\sum_{\mathbf{J}=0,1} A_{\mathbf{J}}\left(\mathbf{r}-\mathbf{R}_{\mathbf{I}(\mathbf{r})}\right)\rho_{\mathbf{I}(\mathbf{r})+\mathbf{J}}d\mathbf{r}. \tag{3}$$

For any lattice vector $\mathbf{R}$ we define the corresponding computational cell as $\mathcal{C}(\mathbf{R})$ which is just the set of points satisfying $R_a \leq r_a < R_a + \Delta_a$. Then, we can break up the integral over all of space into a sum over computational cells gives

$$\begin{aligned}n_{\mathbf{S}}^{(\alpha)} &= \sum_{\mathbf{R}'}\int_{\mathcal{C}(\mathbf{R}')} w^{(\alpha)}(\mathbf{R}_{\mathbf{S}}-\mathbf{r})\sum_{\mathbf{J}=0,1} A_{\mathbf{J}}\left(\mathbf{r}-\mathbf{R}_{\mathbf{I}(\mathbf{r})}\right)\rho_{\mathbf{I}(\mathbf{r})+\mathbf{J}}d\mathbf{r} \\ &= \sum_{\mathbf{R}}\sum_{\mathbf{J}=0,1}\int_{\mathcal{C}(\mathbf{R})} w^{(\alpha)}(\mathbf{R}_{\mathbf{S}}-\mathbf{r})\,A_{\mathbf{J}}(\mathbf{r}-\mathbf{R})\,\rho_{\mathbf{I}(\mathbf{R})+\mathbf{J}}d\mathbf{r}\end{aligned} \tag{4}$$

* http://www.lutsko.com; jlutsko@ulb.ac.be

where the second line follows from noting that if $\mathbf{r} \in \mathcal{C}(\mathbf{R}')$ then $\mathbf{R}_{\mathbf{I}(\mathbf{r})} = \mathbf{R}'$ and $\mathbf{I}(\mathbf{r}) = \mathbf{I}(\mathbf{R}')$ and then renaming the summation variable. The sum over sites $\mathbf{R}$ is equivalent to a sum over indices $\mathbf{K}$ so

$$\begin{aligned} n_{\mathbf{S}}^{(\alpha)} &= \sum_{\mathbf{J}=0,1}\sum_{\mathbf{K}}\int_{\mathcal{C}(\mathbf{R_K})} w^{(\alpha)}(\mathbf{R_S}-\mathbf{r})\, A_{\mathbf{J}}(\mathbf{r}-\mathbf{R_K})\,\rho_{\mathbf{K}+\mathbf{J}}d\mathbf{r} \\ &= \sum_{\mathbf{L}}\rho_{\mathbf{L}}\sum_{\mathbf{J}=0,1}\int_{\mathcal{C}(\mathbf{R_{L-J}})} w^{(\alpha)}(\mathbf{R_S}-\mathbf{r})\, A_{\mathbf{J}}(\mathbf{r}-\mathbf{R_{L-J}})\, d\mathbf{r} \\ &= \sum_{\mathbf{L}}\rho_{\mathbf{L}}\sum_{\mathbf{J}=0,1}\int_{\mathcal{C}(\mathbf{0})} w^{(\alpha)}(\mathbf{R_{S-L+J}}-\mathbf{r})\, A_{\mathbf{J}}(\mathbf{r})\, d\mathbf{r} \end{aligned} \tag{5}$$

so that

$$n_{\mathbf{S}}^{(\alpha)} = \sum_{\mathbf{L}} \widetilde{w}_{\mathbf{S-L}}^{(\alpha)}\rho_{\mathbf{L}} \tag{6}$$

with

$$\widetilde{w}_{\mathbf{S}}^{(\alpha)} = \sum_{\mathbf{J}=0,1}\int_{\mathcal{C}(\mathbf{0})} w^{(\alpha)}(\mathbf{R_{S+J}}-\mathbf{r})\, A_{\mathbf{J}}(\mathbf{r})\, d\mathbf{r} \tag{7}$$

Note that the sum over $\mathbf{I}$ is due to the fact that the density at each lattice site contributes to the interpolation in the 8 computational cells that meet at this point.

### B. Spherical Symmetry reduces computational cost

We first note that all of the weights have a definite parity under the change in sign of their argument: for any vector $\mathbf{r}$ if $\mathcal{R}_j\mathbf{r}$ sends $r_j \to -r_j$ while the other components remain unchanged (i.e. it is a reflection) then from their definitions one has that $w^{(\alpha)}(\mathcal{R}_j\mathbf{r}) = \epsilon_j^{(\alpha)} w^{(\alpha)}(\mathbf{r})$ where $\epsilon_j^{(\eta)} = \epsilon_j^{(s)} = 1$, $\epsilon_j^{(v_i)} = 1 - 2\delta_{ij}$ and $\epsilon_k^{(T_{ij})} = (1-2\delta_{ik})(1-2\delta_{jk})$. This parity extends to the discrete weights $\widetilde{w}$ as follows. Writing the z-specific parts of the general expression explicitly, we need

$$\begin{aligned} &\sum_{J_z=0,1}\int_0^{\Delta_z} w^{(\alpha)}(\ldots(R_{S_z+J_z}-z)\,\widehat{\mathbf{z}})\left(\delta_{J_z0}\left(1-\frac{z}{\Delta_z}\right)+\delta_{J_z1}\frac{z}{\Delta_z}\right)dz \\ &= \int_0^{\Delta_z} w^{(\alpha)}(\ldots(R_{S_z}-z)\,\widehat{\mathbf{z}})\left(1-\frac{z}{\Delta_z}\right)dz + \int_0^{\Delta_z} w^{(\alpha)}(\ldots(R_{S_z}+\Delta_z-z)\,\widehat{\mathbf{z}})\left(\frac{z}{\Delta_z}\right)dz \\ &= \epsilon_j^{(\alpha)}\int_0^{\Delta_z} w^{(\alpha)}(\ldots(-R_{S_z}+z)\,\widehat{\mathbf{z}})\left(1-\frac{z}{\Delta_z}\right)dz + \epsilon_j^{(\alpha)}\int_0^{\Delta_z} w^{(\alpha)}(\ldots(-R_{S_z}-\Delta_z+z)\,\widehat{\mathbf{z}})\left(\frac{z}{\Delta_z}\right)dz \\ &= \epsilon_j^{(\alpha)}\int_0^{\Delta_z} w^{(\alpha)}(\ldots(R_{-S_z}+\Delta_z-z)\,\widehat{\mathbf{z}})\left(\frac{z}{\Delta_z}\right)dz + \epsilon_j^{(\alpha)}\int_0^{\Delta_z} w^{(\alpha)}(\ldots(-R_{S_z}-z)\,\widehat{\mathbf{z}})\left(1-\frac{z}{\Delta_z}\right)dz \\ &= \epsilon_j^{(\alpha)}\sum_{J_z=0,1}\int_0^{\Delta_z} w^{(\alpha)}(\ldots(R_{-S_z+J_z}-z)\,\widehat{\mathbf{z}})\left(\delta_{J_z0}\left(1-\frac{z}{\Delta_z}\right)+\delta_{J_z1}\frac{z}{\Delta_z}\right)dz \end{aligned} \tag{8}$$

where the third line results from the use of parity in the form $w^{(\alpha)}(\mathbf{r}) = \epsilon_j^{(\alpha)} w^{(\alpha)}(\mathcal{R}_j\mathbf{r})$ and the fourth from a change of integration variable. This shows that , in general, $\widetilde{w}^{(\alpha)}(\mathbf{S}) = \epsilon_j^{(\alpha)}\widetilde{w}^{(\alpha)}(\mathcal{R}_j\mathbf{S})$ meaning that the weights need only be computed in the positive octant of the sphere.

### C. General framework for the evaluations

In the remainer of this development we specialize to the special case $\Delta_x = \Delta_y = \Delta_z = \Delta$ and furthermore we express all distances in terms of $\Delta$ (so, in effect, we use units such that $\Delta = 1$). This means in particular that

$\mathbf{R_I} = \Delta_x I_x \widehat{\mathbf{x}} + \Delta_y I_y \widehat{\mathbf{y}} + \Delta_z I_z \widehat{\mathbf{z}} \to \Delta \left( I_x \widehat{\mathbf{x}} + I_y \widehat{\mathbf{y}} + I_z \widehat{\mathbf{z}} \right) \to I_x \widehat{\mathbf{x}} + I_y \widehat{\mathbf{y}} + I_z \widehat{\mathbf{z}}$ or, in brief, $\mathbf{R_I} \to \mathbf{I}$. The interpolation matrix becomes

$$A_{\mathbf{J}}\left(\mathbf{r}\right) = \prod_{a=x,y,z} \left( \left(1 - r_a\right) \delta_{J_a=0} + r_a \delta_{J_a=1} \right) = \prod_{a=x,y,z} \left( \left(1 - 2r_a\right) \delta_{J_a=0} + r_a \right) \tag{9}$$

and we can write the expressions for the discrete weights as

$$\begin{aligned} \widetilde{w}^{(\alpha)}\left(\mathbf{S}\right) &= \sum_{\mathbf{J}=0,1} \int_{\mathcal{C}(\mathbf{0})} w^{(\alpha)}\left(\mathbf{R}_{\mathbf{S}+\mathbf{J}} - \mathbf{r}\right) A_{\mathbf{J}}\left(\mathbf{r}\right) d\mathbf{r} \\ &= \sum_{\mathbf{J}=0,1} \int_0^{\mathbf{1}} w^{(\alpha)}\left(\mathbf{S} + \mathbf{J} - \mathbf{r}\right) \prod_{a=x,y,z} \left( \left(1 - r_a\right) \delta_{J_a 0} + r_a \delta_{J_a 1} \right) d\mathbf{r} \\ &= \sum_{\mathbf{J}\in\{0,1\}} \int_{\mathbf{S}+\mathbf{J}-\mathbf{1}}^{\mathbf{S}+\mathbf{J}} w^{(\alpha)}\left(\mathbf{s}\right) \prod_{a=x,y,z} \left( \left(1 - S_a + s_a\right) \delta_{J_a 0} + \left(S_a + 1 - s_a\right) \delta_{J_a 1} \right) d\mathbf{s} \end{aligned} \tag{10}$$

To clarify a little, consider a single component and expand the sum

$$\begin{aligned} &\int_{S_x-1}^{S_x} w^{(\alpha)}\left(\mathbf{s}\right) \left(1 - S_x + s_x\right) ds_x + \int_{S_x}^{S_x+1} w^{(\alpha)}\left(\mathbf{s}\right) \left(S_x + 1 - s_x\right) ds_x \\ &= \sum_{I_x=-1,1} \int_{S_x}^{S_x+I_x} w^{(\alpha)}\left(\mathbf{s}\right) \left(S_x + I_x - s_x\right) ds_x \end{aligned} \tag{11}$$

so we can write

$$\widetilde{w}^{(\alpha)}\left(\mathbf{S}\right) = \sum_{\mathbf{I}\in\{-1,1\}} J^{(\alpha)}\left(\mathbf{S} + \mathbf{I}, \mathbf{I}\right) \tag{12}$$

with

$$J^{(\alpha)}\left(\mathbf{T}, \mathbf{I}\right) = \int_{\mathbf{T}-\mathbf{I}}^{\mathbf{T}} w^{(\alpha)}\left(\mathbf{s}\right) \prod_{j=x,y,z} \left(T_j - s_j\right) d\mathbf{s}. \tag{13}$$

In the following, it will be convenient to assume that $S_j + I_j = S_j \pm 1 \geq 0$.We already know that we can restrict the calculations to the case $S_j \geq 0$ due to the spherical symmetry so the only problem with this condition occurs when $S_j = 0$. In that case, we will be evaluating

$$\begin{aligned} &\int_0^1 w^{(\alpha)}\left(\mathbf{s}\right) \left(1 - s_j\right) ds_j + \int_0^{-1} w^{(\alpha)}\left(\mathbf{s}\right) \left(-1 - s_j\right) ds_j \\ &= \int_0^1 w^{(\alpha)}\left(\mathbf{s}\right) \left(1 - s_j\right) ds_j - \int_0^1 w^{(\alpha)}\left(\mathcal{R}_j \mathbf{s}\right) \left(-1 + s_j\right) ds_j \\ &= \left(1 + \epsilon_j^{(\alpha)}\right) \int_0^1 w^{(\alpha)}\left(\mathbf{s}\right) \left(1 - s_j\right) ds_j \end{aligned} \tag{14}$$

This means that in the evaluation of $\widetilde{w}^{(\alpha)}\left(\mathbf{S}\right)$, whenever $S_j$ is zero, we should replace the contribution of $I_j = -1$ by $\epsilon_j^{(\alpha)}$ times that of $I_j = 1$.

### D. Evaluation of local packing fraction

We now specialize to the local packing fraction so that we need

$$J^{(\eta)}\left(\mathbf{T}, \mathbf{I}\right) = \int_{\mathbf{T}-\mathbf{I}}^{\mathbf{T}} \Theta\left(R - s\right) \prod_{j=x,y,z} \left(T_j - s_j\right) d\mathbf{s}. \tag{15}$$

From the preceding discussion, it is sufficient to limit attention to the cases for which $T_j \geq 0$. In the following, we will make extensive use of the identity valid for any reasonable function $g(z)$

$$\int_a^b g(z)\,\Theta(W-z)\,dz = \sum_{d=a,b} \Theta(W-d)\left(\delta_{d=b}-\delta_{d=a}\right)\int_W^d g(z)\,dz \tag{16}$$

which is verified by differentiation and noting that the right hand side vanishes when $b=a$.

We write $J$ as

$$J^{(\eta)}(\mathbf{T},\mathbf{I}) = \int_{T_x-I_x}^{T_x}\left(\int_{T_y-I_y}^{T_y}\left(\int_{T_z-I_z}^{T_z}\Theta(R-s)(T_z-s_z)\,dz\right)(T_y-s_y)\,dy\right)(T_x-s_x)\,dx \tag{17}$$

or

$$\begin{aligned} J^{(\eta)}(\mathbf{S},\mathbf{I}) &= \int_{T_x-I_x}^{T_x} J_y^{(\eta)}(s_x)(T_x-s_x)\,dx \\ J_y^{(\eta)}(s_x) &= \int_{T_y-I_y}^{T_y} J_z^{(\eta)}(s_x,s_y)(T_y-s_y)\,dy \\ J_z^{(\eta)}(s_x,s_y) &= \int_{T_z-I_z}^{T_z}\Theta\left(\sqrt{R^2-s_x^2-s_y^2}-s_z\right)(T_z-s_z)\,dz \end{aligned} \tag{18}$$

So, using the identity above,

$$\begin{aligned} J_z^{(\eta)}(s_x,s_y) &= \int_{T_z-I_z}^{T_z}\Theta\left(\sqrt{R^2-s_x^2-s_y^2}-s_z\right)(T_z-s_z)\,dz \\ &= \frac{1}{2}\sum_{V_z=T_z-I_z,T_z}\Theta\left(\sqrt{R^2-s_x^2-s_y^2}-V_z\right)\left(\delta_{V_z=T_z}-\delta_{V_z=T_z-I_z}\right)F_z(s_x,s_y,V_z) \end{aligned} \tag{19}$$

with

$$F_z^{(\eta)}(s_x,s_y,V_z) = 2\int_{\sqrt{R^2-s_x^2-s_y^2}}^{V_z}(T_z-z)\,dz \tag{20}$$

where the factor of $-2$ is included for later convenience. Then

$$\begin{aligned} J_y^{(\eta)}(s_x) &= \sum_{V_z=T_z-I_z,T_z}\left(\delta_{V_z=T_z}-\delta_{V_z=T_z-I_z}\right)\int_{T_y-I_y}^{T_y}\Theta\left(\sqrt{R^2-s_x^2-s_y^2}-V_z\right)F_z(s_x,s_y,V_z)(T_y-s_y)\,dy \\ &= \sum_{V_z=T_z-I_z,T_z}\left(\delta_{V_z=T_z}-\delta_{V_z=T_z-I_z}\right)\int_{T_y-I_y}^{T_y}\Theta\left(\sqrt{R^2-s_x^2-V_z^2}-s_y\right)F_z(s_x,s_y,V_z)(T_y-s_y)\,dy \\ &= \sum_{V_z=T_z-I_z,T_z}\left(\delta_{V_z=T_z}-\delta_{V_z=T_z-I_z}\right)\sum_{V_y=T_y-I_y,T_y}\Theta\left(\sqrt{R^2-s_x^2-V_z^2}-V_y\right)\left(\delta_{V_y=T_y}-\delta_{V_y=T_y-I_y}\right)F_y(s_x,V_y,V_z) \end{aligned} \tag{21}$$

with

$$F_y^{(\eta)}(s_x,V_y,V_z) = \int_{\sqrt{R^2-s_x^2-V_z^2}}^{V_y}(T_y-y)\,F_z^{(\eta)}(s_x,y,V_z)\,dy \tag{22}$$

And finally,

$$J^{(\eta)}\left(\mathbf{T},\mathbf{I}\right)=\sum_{V_z=T_z-I_z,T_z}\left(\delta_{V_z=T_z}-\delta_{V_z=T_z-I_z}\right)\sum_{V_y=T_y-I_y,T_y}\left(\delta_{V_y=T_y}-\delta_{V_y=T_y-I_y}\right)$$
$$\times\int_{T_x-I_x}^{T_x}\Theta\left(\sqrt{R^2-s_x^2-V_z^2}-V_y\right)F_y\left(x,V_y,V_z\right)\left(T_x-x\right)dx$$
$$=\sum_{V_z=T_z-I_z,T_z}\left(\delta_{V_z=T_z}-\delta_{V_z=T_z-I_z}\right)\sum_{V_y=T_y-I_y,T_y}\left(\delta_{V_y=T_y}-\delta_{V_y=T_y-I_y}\right)$$
$$\times\int_{T_x-I_x}^{T_x}\Theta\left(\sqrt{R^2-V_y^2-V_z^2}-s_x\right)F_y\left(x,V_y,V_z\right)\left(T_x-x\right)dx$$
$$=\sum_{\mathbf{V}=\mathbf{T}-\mathbf{I},\mathbf{T}}\prod_{a=x,y,z}\left(\delta_{V_a=T_a}-\delta_{V_a=T_a-I_a}\right)\Theta\left(\sqrt{R^2-V_y^2-V_z^2}-V_x\right)F\left(\mathbf{V}\right) \quad (23)$$

with

$$F^{(\eta)}\left(\mathbf{V}\right)=\int_{\sqrt{R^2-V_y^2-V_z^2}}^{V_x}\left(T_x-x\right)F_y^{(\eta)}\left(x,V_y,V_z\right)dx. \quad (24)$$

In summary

$$J^{(\eta)}\left(\mathbf{T},\mathbf{I}\right)=\frac{1}{2}\sum_{\mathbf{V}=\mathbf{T}-\mathbf{I},\mathbf{T}}\Theta\left(R-V\right)\prod_{a=x,y,z}\left(\delta_{V_a=T_a}-\delta_{V_a=T_a-I_a}\right)F^{(\eta)}\left(\mathbf{V}\right) \quad (25)$$
$$F^{(\eta)}\left(\mathbf{V}\right)=\int_{\sqrt{R^2-V_y^2-V_z^2}}^{V_x}\left(T_x-x\right)F_y^{(\eta)}\left(x,V_y,V_z\right)dx$$
$$F_y^{(\eta)}\left(s_x,V_y,V_z\right)=\int_{\sqrt{R^2-s_x^2-V_z^2}}^{V_y}\left(T_y-y\right)F_z^{(\eta)}\left(s_x,y,V_z\right)dy$$
$$F_z^{(\eta)}\left(s_x,s_y,V_z\right)=2\int_{\sqrt{R^2-s_x^2-s_y^2}}^{V_z}\left(T_z-z\right)dz$$

### E. Evaluation of surface measures

We start with $w^{(s)}(\mathbf{r})$ for which we need

$$J^{(s)}\left(\mathbf{T},\mathbf{I}\right)=\int_{\mathbf{T}-\mathbf{I}}^{\mathbf{T}}\delta\left(R-s\right)\prod_{j=x,y,z}\left(T_j-s_j\right)d\mathbf{s}. \quad (26)$$

Again, we assime that $T_j\geq 0$. Next, this is written as

$$J^{(s)}\left(\mathbf{T},\mathbf{I}\right)=\int_{T_x-I_x}^{T_x}\left(\int_{T_y-I_y}^{T_y}\left(\int_{T_z-I_z}^{T_z}\delta\left(R-s\right)\left(T_z-s_z\right)dz\right)\left(T_y-s_y\right)dy\right)\left(T_x-s_x\right)dx \quad (27)$$

or

$$J^{(s)}\left(\mathbf{S},\mathbf{I}\right)=\int_{T_x-I_x}^{T_x}J_y\left(s_x\right)\left(T_x-s_x\right)dx \quad (28)$$
$$J_y\left(s_x\right)=\int_{T_y-I_y}^{T_y}J_z\left(s_x,s_y\right)\left(T_y-s_y\right)dy$$
$$J_z\left(s_x,s_y\right)=\int_{T_z-I_z}^{T_z}\delta\left(R-\sqrt{s_x^2+s_y^2+s_z^2}\right)\left(T_z-s_z\right)dz$$

Now,

$$J_z(s_x,s_y)=\int_{T_z-I_z}^{T_z}\frac{R}{|s_z|}\delta\left(\sqrt{R^2-s_x^2-s_y^2}-s_z\right)(T_z-s_z)\,dz \tag{29}$$
$$=\frac{R}{\sqrt{R^2-s_x^2-s_y^2}}\left(T_z-\sqrt{R^2-s_x^2-s_y^2}\right)\left[\begin{array}{c}\Theta(I_z)\,\Theta\left(T_z-\sqrt{R^2-s_x^2-s_y^2}\right)\Theta\left(\sqrt{R^2-s_x^2-s_y^2}-(T_z-I_z)\right)\\ -\Theta(-I_z)\,\Theta\left(T_z-I_z-\sqrt{R^2-s_x^2-s_y^2}\right)\Theta\left(\sqrt{R^2-s_x^2-s_y^2}-T_z\right)\end{array}\right]$$

Recall that we are working under the assumption that $I_z=\pm1$ so

$$\Theta(I_z)\,\Theta\left(T_z-\sqrt{R^2-s_x^2-s_y^2}\right)\Theta\left(\sqrt{R^2-s_x^2-s_y^2}-(T_z-I_z)\right) \tag{30}$$
$$=\Theta(I_z)\left[\Theta\left(\sqrt{R^2-s_x^2-s_y^2}-(T_z-I_z)\right)-\Theta\left(\sqrt{R^2-s_x^2-s_y^2}-T_z\right)\right]$$

and

$$\Theta(-I_z)\,\Theta\left(T_z-I_z-\sqrt{R^2-s_x^2-s_y^2}\right)\Theta\left(\sqrt{R^2-s_x^2-s_y^2}-T_z\right) \tag{31}$$
$$=\Theta(-I_z)\left[\Theta\left(\sqrt{R^2-s_x^2-s_y^2}-T_z\right)-\Theta\left(\sqrt{R^2-s_x^2-s_y^2}-(T_z-I_z)\right)\right]$$

allowing us to write

$$J_z(s_x,s_y)=\frac{R}{\sqrt{R^2-s_x^2-s_y^2}}\left(T_z-\sqrt{R^2-s_x^2-s_y^2}\right)\left[\Theta\left(\sqrt{R^2-s_x^2-s_y^2}-(T_z-I_z)\right)-\Theta\left(\sqrt{R^2-s_x^2-s_y^2}-T_z\right)\right] \tag{32}$$
$$=-\sum_{V_z=T_z-I_z,T_z}\Theta\left(\sqrt{R^2-s_x^2-s_y^2}-V_z\right)\left(\delta_{V_z=T_z}-\delta_{V_z=T_z-I_z}\right)\frac{R}{\sqrt{R^2-s_x^2-s_y^2}}\left(T_z-\sqrt{R^2-s_x^2-s_y^2}\right)$$

From this point, the development is exactly as above resulting in

$$J^{(s)}(\mathbf{T},\mathbf{I})=\sum_{\mathbf{V}=\mathbf{T}-\mathbf{I},\mathbf{T}}\Theta(R-V)\prod_i\left(\delta_{V_i=T_i}-\delta_{V_i=T_i-I_i}\right)F^{(s)}(\mathbf{V}) \tag{33}$$
$$F^{(s)}(\mathbf{V})=\int_{\sqrt{R^2-V_y^2-V_z^2}}^{V_x}(T_x-x)\,F_y^{(s)}(x,V_y,V_z)\,dx$$
$$F_y^{(s)}(s_x,V_y,V_z)=\int_{\sqrt{R^2-s_x^2-V_z^2}}^{V_y}(T_y-y)\,F_z^{(s)}(s_x,y,V_z)\,dy$$
$$F_z^{(s)}(s_x,s_y,V_z)=-R\left(\frac{T_z}{\sqrt{R^2-s_x^2-s_y^2}}-1\right)$$

Clearly, the others follow with

$$F_z^{(s)}(s_x,s_y,V_z)=F_z^{(v_x)}(s_x,s_y,V_z)=F_z^{(T_{xx})}(s_x,s_y,V_z)=F_z^{(T_{xy})}(s_x,s_y,V_z) \tag{34}$$
$$F_y^{(s)}(s_x,s_y,V_z)=F_y^{(v_x)}(s_x,s_y,V_z)=F_y^{(T_{xx})}(s_x,s_y,V_z)$$

and

$$F_y^{(T_{xy})}(s_x,V_y,V_z)=\int_{\sqrt{R^2-s_x^2-V_z^2}}^{V_y}(T_y-y)\,yF_z^{(s)}(s_x,y,V_z)\,dy \tag{35}$$
$$F^{(v_x)}(\mathbf{V})=R^{-1}\int_{\sqrt{R^2-V_y^2-V_z^2}}^{V_x}(T_x-x)\,xF_y^{(s)}(x,V_y,V_z)\,dx$$
$$F^{(T_{xx})}(\mathbf{V})=R^{-2}\int_{\sqrt{R^2-V_y^2-V_z^2}}^{V_x}(T_x-x)\,x^2F_y^{(s)}(x,V_y,V_z)\,dx$$
$$F^{(T_{xy})}(\mathbf{V})=R^{-2}\int_{\sqrt{R^2-V_y^2-V_z^2}}^{V_x}(T_x-x)\,xF_y^{(T_{xy})}(x,V_y,V_z)\,dx$$

### F. Explicit formulae

#### 1. Integrals

The evaluations will be written in terms of the integrals

$$
\begin{aligned}
I_0\left(X;A\right) &= \int \sqrt{A-X^2}dX = \frac{1}{2}X\sqrt{A-X^2}+\frac{1}{2}A\arcsin\frac{X}{\sqrt{A}} \\
I_1\left(X;A\right) &= \int X\sqrt{A-X^2}dX = -\frac{1}{3}\left(A-X^2\right)\sqrt{A-X^2} \\
I_2\left(X;A\right) &= \int X^2\sqrt{A-X^2}dX = \frac{1}{8}X\left(2X^2-A\right)\sqrt{A-X^2}+\frac{1}{8}A^2\arcsin\frac{X}{\sqrt{A}} \\
I_3\left(X;A\right) &= \int X^3\sqrt{A-X^2}dX = -\frac{1}{15}\left(A-X^2\right)\left(3X^2+2A\right)\sqrt{A-X^2} \\
I_4\left(X;A\right) &= \int X^4\sqrt{A-X^2}dX = \frac{1}{48}\left(8X^4-2AX^2-3A^2\right)X\sqrt{A-X^2}+\frac{1}{16}A^3\arctan\frac{X}{\sqrt{A-X^2}} \\
K\left(X;V\right) &= \int \frac{1}{\left(R^2-X^2\right)\sqrt{R^2-X^2-V^2}}dX = \frac{1}{RV}\arcsin\frac{VX}{\sqrt{\left(R^2-V^2\right)\left(R^2-X^2\right)}}
\end{aligned}
\tag{36}
$$

and

$$
\begin{aligned}
J_0\left(X;V\right) &= \int \arcsin\frac{V}{\sqrt{R^2-X^2}}dX = X\arcsin\frac{V}{\sqrt{R^2-X^2}}+V\arcsin\frac{X}{\sqrt{R^2-V^2}}-R\arcsin\frac{VX}{\sqrt{\left(R^2-V^2\right)\left(R^2-X^2\right)}} \\
J_1\left(X;V\right) &= \int X\arcsin\frac{V}{\sqrt{R^2-X^2}}dX = -\frac{1}{2}V\sqrt{R^2-V^2-X^2}+\frac{1}{2}\left(X^2-R^2\right)\arcsin\frac{V}{\sqrt{R^2-X^2}} \\
J_2\left(X;V\right) &= \int X^2\arcsin\frac{V}{\sqrt{R^2-X^2}}dX = -\frac{1}{6}V\left(V^2-3R^2\right)\arcsin\frac{X}{\sqrt{R^2-V^2}}+\frac{1}{3}X^3\arcsin\frac{V}{\sqrt{R^2-X^2}} \\
&\quad -\frac{1}{3}R^3\arcsin\frac{XV}{\sqrt{\left(R^2-X^2\right)\left(R^2-V^2\right)}}-\frac{1}{6}VX\sqrt{R^2-X^2-V^2} \\
J_3\left(X;V\right) &= \int X^3\arcsin\frac{V}{\sqrt{R^2-X^2}}dX = \frac{1}{4}\left(X^4-R^4\right)\arcsin\frac{V}{\sqrt{R^2-X^2}}+\frac{\pi}{8}R^4-\frac{V}{12}\left(5R^2+X^2-2V^2\right)\sqrt{R^2-V^2-X^2} \\
J_4\left(X;V\right) &= \int X^4\arcsin\frac{V}{\sqrt{R^2-X^2}}dX = \frac{1}{40}VX\left(3V^2-2X^2-7R^2\right)\sqrt{R^2-V^2-X^2} \\
&\quad +\frac{1}{40}V\left(3V^4-10V^2R^2+15R^4\right)\arcsin\frac{X}{\sqrt{R^2-V^2}}+\frac{1}{5}X^5\arcsin\frac{V}{\sqrt{R^2-X^2}} \\
&\quad -\frac{1}{5}R^5\arcsin\frac{XV}{\sqrt{\left(R^2-X^2\right)\left(R^2-V^2\right)}}
\end{aligned}
\tag{37}
$$

#### 2. Packing fraction

We have

$$
\begin{aligned}
J^{(\eta)}\left(\mathbf{T},\mathbf{I}\right) &= \sum_{\mathbf{V}=\mathbf{T}-\mathbf{I},\mathbf{T}}\Theta\left(R-V\right)\prod_i\left(\delta_{V_i=T_i}-\delta_{V_i=T_i-I_i}\right)F\left(\mathbf{V}\right) \\
F^{(\eta)}\left(\mathbf{V}\right) &= \int_{\sqrt{R^2-V_y^2-V_z^2}}^{V_x}\left(T_x-x\right)F_y\left(x,V_y,V_z\right)dx \\
F_y^{(\eta)}\left(s_x,V_y,V_z\right) &= \int_{\sqrt{R^2-s_x^2-V_z^2}}^{V_y}\left(T_y-y\right)F_z\left(s_x,y,V_z\right)dy \\
F_z^{(\eta)}\left(s_x,s_y,V_z\right) &= \int_{\sqrt{R^2-s_x^2-s_y^2}}^{V_z}\left(T_z-z\right)dz
\end{aligned}
\tag{38}
$$

Now,

$$F_z^{(\eta)}(s_x,s_y,V_z)=\frac{1}{2}\left(R^2-s_x^2-s_y^2\right)+T_zV_z-\frac{1}{2}V_z^2-T_z\sqrt{R^2-s_x^2-s_y^2} \tag{39}$$

and

$$F_y^{(\eta)}(s_x,V_y,V_z)=\int_{\sqrt{R^2-s_x^2-V_z^2}}^{V_y}(T_y-y)\left[\frac{1}{2}R^2-\frac{1}{2}s_x^2-\frac{1}{2}y^2+T_zV_z-\frac{1}{2}V_z^2-T_z\sqrt{R^2-s_x^2-y^2}\right]dy \tag{40}$$

This evaluates to

$$\begin{aligned}F_y^{(\eta)}(s_x,V_y,V_z)=&\,T_yT_zV_yV_z+\frac{1}{4}V_y^2V_z^2+\frac{1}{8}\left(R^2-s_x^2\right)^2\\&-\frac{1}{6}T_yV_y^3-\frac{1}{6}T_zV_z^3-\frac{1}{2}T_zV_zV_y^2-\frac{1}{2}T_yV_yV_z^2+\frac{1}{8}V_y^4+\frac{1}{8}V_z^4\\&+\frac{1}{2}\left(T_yV_y+T_zV_z-\frac{1}{2}V_y^2-\frac{1}{2}V_z^2+\frac{\pi}{2}T_yT_z\right)\left(R^2-s_x^2\right)\\&-\frac{1}{2}T_yT_z\left(R^2-s_x^2\right)\left(\arcsin\left(\frac{V_y}{\sqrt{R^2-s_x^2}}\right)+\arcsin\left(\frac{V_z}{\sqrt{R^2-s_x^2}}\right)\right)\\&-\left(\frac{1}{2}T_yV_y+\frac{1}{3}\left(R^2-s_x^2-V_y^2\right)\right)T_z\sqrt{R^2-s_x^2-V_y^2}-\left(\frac{1}{2}T_zV_z+\frac{1}{3}\left(R^2-s_x^2-V_z^2\right)\right)T_y\sqrt{R^2-s_x^2-V_z^2}\end{aligned} \tag{41}$$

as can be checked by differentiating with respect to $V_y$ and verifying that it vanishes when $V_y=\sqrt{R^2-s_x^2-V_z^2}$. We rewrite this as

$$\begin{aligned}F_y^{(\eta)}(x,V_y,V_z)=&\,T_yT_zV_yV_z+\frac{1}{4}V_y^2V_z^2+\frac{1}{8}R^4-\frac{1}{6}T_yV_y^3-\frac{1}{6}T_zV_z^3-\frac{1}{2}T_zV_zV_y^2-\frac{1}{2}T_yV_yV_z^2\\&+\frac{1}{8}V_y^4+\frac{1}{8}V_z^4+\frac{1}{2}R^2\left(T_yV_y+T_zV_z-\frac{1}{2}V_y^2-\frac{1}{2}V_z^2+\frac{\pi}{2}T_yT_z\right)\\&-\frac{1}{2}\left(T_yV_y+T_zV_z-\frac{1}{2}V_y^2-\frac{1}{2}V_z^2+\frac{\pi}{2}T_yT_z+\frac{1}{2}R^2\right)x^2+\frac{1}{8}x^4\\&-\frac{1}{2}T_yT_z\left(R^2-x^2\right)\left(\arcsin\left(\frac{V_y}{\sqrt{R^2-x^2}}\right)+\arcsin\left(\frac{V_z}{\sqrt{R^2-x^2}}\right)\right)\\&-\left(\frac{1}{2}T_yV_y+\frac{1}{3}\left(R^2-V_y^2\right)-\frac{1}{3}x^2\right)T_z\sqrt{R^2-x^2-V_y^2}-\left(\frac{1}{2}T_zV_z+\frac{1}{3}\left(R^2-V_z^2\right)-\frac{1}{3}x^2\right)T_y\sqrt{R^2-x^2-V_z^2}\end{aligned} \tag{42}$$

with

$$\begin{aligned}A=&\,T_yT_zV_yV_z+\frac{1}{4}V_y^2V_z^2+\frac{1}{8}R^4-\frac{1}{6}T_yV_y^3-\frac{1}{6}T_zV_z^3-\frac{1}{2}T_zV_zV_y^2-\frac{1}{2}T_yV_yV_z^2\\&+\frac{1}{8}V_y^4+\frac{1}{8}V_z^4+\frac{1}{2}R^2\left(T_yV_y+T_zV_z-\frac{1}{2}V_y^2-\frac{1}{2}V_z^2+\frac{\pi}{2}T_yT_z\right)\\B=&\,\frac{1}{2}T_yV_y+\frac{1}{2}T_zV_z-\frac{1}{4}V_y^2-\frac{1}{4}V_z^2+\frac{\pi}{4}T_yT_z+\frac{1}{4}R^2\\C=&\,\frac{1}{2}T_yV_y+\frac{1}{3}\left(R^2-V_y^2\right)\\D=&\,\frac{1}{2}T_zV_z+\frac{1}{3}\left(R^2-V_z^2\right)\end{aligned} \tag{43}$$

so

$$\begin{aligned}(T_x-x)\,F_y^{(\eta)}(x,V_y,V_z)=&\,T_xA-Ax-x^2T_xB+x^3B+\frac{1}{8}T_xx^4-\frac{1}{8}x^5\\&-\frac{1}{2}T_yT_z\left(T_xR^2-xR^2-x^2T_x+x^3\right)\left(\arcsin\left(\frac{V_y}{\sqrt{R^2-x^2}}\right)+\arcsin\left(\frac{V_z}{\sqrt{R^2-x^2}}\right)\right)\\&-\left(T_xT_zC-T_zCx-\frac{1}{3}T_xT_zx^2+\frac{1}{3}T_zx^3\right)\sqrt{R^2-x^2-V_y^2}\\&-\left(T_xT_yD-T_yDx-\frac{1}{3}T_xT_yx^2+\frac{1}{3}T_yx^3\right)\sqrt{R^2-x^2-V_z^2}\end{aligned} \tag{44}$$

and finally

$$F^{(\eta)}(\mathbf{V}) = G^{(\eta)}(V_x) - G^{(\eta)}\left(\sqrt{R^2 - V_y^2 - V_z^2}\right) \tag{45}$$

with

$$\begin{aligned} G^{(\eta)}(X, V_y, V_z) = {} & T_x A X - \frac{1}{2} A x X^2 - \frac{1}{3} X^3 T_x B + \frac{1}{4} X^4 B + \frac{1}{40} T_x X^5 - \frac{1}{48} X^6 \\ & - \frac{1}{2} T_y T_z \left(T_x R^2 J_0(X; V_y) - R^2 J_1(X; V_y) - T_x J_2(X; V_y) + J_3(X; V_y)\right) \\ & - \frac{1}{2} T_y T_z \left(T_x R^2 J_0(X; V_z) - R^2 J_1(X; V_z) - T_x J_2(X; V_z) + J_3(X; V_z)\right) \\ & - \left(T_x T_z C I_0\left(X; \sqrt{R^2 - V_y^2}\right) - T_z C I_1\left(X; \sqrt{R^2 - V_y^2}\right) - \frac{1}{3} T_x T_z I_2\left(X; \sqrt{R^2 - V_y^2}\right) + \frac{1}{3} T_z I_3\left(X; \sqrt{R^2 - V_y^2}\right)\right) \\ & - \left(T_x T_y D I_0\left(X; \sqrt{R^2 - V_z^2}\right) - T_y D I_1\left(X; \sqrt{R^2 - V_z^2}\right) - \frac{1}{3} T_x T_y I_2\left(X; \sqrt{R^2 - V_z^2}\right) + \frac{1}{3} T_y I_3\left(X; \sqrt{R^2 - V_z^2}\right)\right) \end{aligned} \tag{46}$$

### *3. Scalar, vector and diagonal tensor element*

We need

$$\begin{aligned} J^{(s)}(\mathbf{T}, \mathbf{I}) &= \sum_{\mathbf{V}=\mathbf{T}-\mathbf{I},\mathbf{T}} \Theta(R - V) \prod_i \left(\delta_{V_i = T_i} - \delta_{V_i = T_i - I_i}\right) F^{(s)}(\mathbf{V}) \\ F^{(s)}(\mathbf{V}) &= G(V_x, V_y, V_z) - G\left(\sqrt{R^2 - V_y^2 - V_z^2}, V_y, V_z\right) \\ G^{(s)}(X, V_y, V_z) &= \int^X (T_x - x) F_y^{(s)}(x, V_y, V_z)\, dx \\ F_y^{(s)}(s_x, V_y, V_z) &= \int_{\sqrt{R^2 - s_x^2 - V_z^2}}^{V_y} (T_y - y) F_z^{(s)}(s_x, y, V_z)\, dy \\ F_z^{(s)}(s_x, s_y, V_z) &= R\left(1 - \frac{T_z}{\sqrt{R^2 - s_x^2 - s_y^2}}\right) \end{aligned} \tag{47}$$

So

$$\begin{aligned} F_y^{(s)}(s_x, V_y, V_z) &= R \int_{\sqrt{R^2 - s_x^2 - V_z^2}}^{V_y} (T_y - y)\left(1 - \frac{T_z}{\sqrt{R^2 - s_x^2 - y^2}}\right) dy \\ &= -R T_y T_z \left(\arcsin\frac{V_y}{\sqrt{R^2 - s_x^2}} + \arcsin\frac{V_z}{\sqrt{R^2 - s_x^2}}\right) \\ &\quad - R T_z \sqrt{R^2 - s_x^2 - V_y^2} - R T_y \sqrt{R^2 - s_x^2 - V_z^2} \\ &\quad + R\left(T_y V_y + T_z V_z - \frac{1}{2} V_y^2 - \frac{1}{2} V_z^2 + \frac{1}{2} R^2 + \frac{\pi}{2} T_y T_z - \frac{1}{2} s_x^2\right) \end{aligned} \tag{48}$$

and if

$$A = T_y V_y + T_z V_z - \frac{1}{2} V_y^2 - \frac{1}{2} V_z^2 + \frac{1}{2} R^2 + \frac{\pi}{2} T_y T_z \tag{49}$$

then

$$\begin{aligned} G^{(s)}\left(X,V_y,V_z\right) = & \frac{1}{8}RX^4 - \frac{1}{6}RT_xX^3 - \frac{1}{2}ARX^2 + AT_xRX \\ & - RT_z\left(T_xI_0\left(X;\sqrt{R^2-V_y^2}\right) - I_1\left(X;\sqrt{R^2-V_y^2}\right)\right) \\ & - RT_y\left(T_xI_0\left(X;\sqrt{R^2-V_z^2}\right) - I_1\left(X;\sqrt{R^2-V_z^2}\right)\right) \\ & - RT_yT_z\left(T_xJ_0\left(X;V_y\right) - J_1\left(X;V_y\right)\right) \\ & - RT_yT_z\left(T_xJ_0\left(X;V_z\right) - J_1\left(X;V_z\right)\right) \end{aligned} \tag{50}$$

From these, we immediately get

$$\begin{aligned} G^{(v_x)}\left(X,V_y,V_z\right) = & \frac{1}{10}RX^5 - \frac{1}{8}RT_xX^4 - \frac{1}{3}ARX^3 + \frac{1}{2}AT_xRX^2 \\ & - RT_z\left(T_xI_1\left(X;\sqrt{R^2-V_y^2}\right) - I_2\left(X;\sqrt{R^2-V_y^2}\right)\right) \\ & - RT_y\left(T_xI_1\left(X;\sqrt{R^2-V_z^2}\right) - I_2\left(X;\sqrt{R^2-V_z^2}\right)\right) \\ & - RT_yT_z\left(T_xJ_1\left(X;V_y\right) - J_2\left(X;V_y\right)\right) \\ & - RT_yT_z\left(T_xJ_1\left(X;V_z\right) - J_2\left(X;V_z\right)\right) \end{aligned} \tag{51}$$

and

$$\begin{aligned} G^{(T_{xx})}\left(X,V_y,V_z\right) = & \frac{1}{12}RX^6 - \frac{1}{10}RT_xX^5 - \frac{1}{4}ARX^4 + \frac{1}{3}AT_xRX^3 \\ & - RT_z\left(T_xI_2\left(X;\sqrt{R^2-V_y^2}\right) - I_3\left(X;\sqrt{R^2-V_y^2}\right)\right) \\ & - RT_y\left(T_xI_2\left(X;\sqrt{R^2-V_z^2}\right) - I_3\left(X;\sqrt{R^2-V_z^2}\right)\right) \\ & - RT_yT_z\left(T_xJ_2\left(X;V_y\right) - J_3\left(X;V_y\right)\right) \\ & - RT_yT_z\left(T_xJ_2\left(X;V_z\right) - J_3\left(X;V_z\right)\right) \end{aligned} \tag{52}$$

### *4. Off diagonal tensor element*

Here we need

$$\begin{aligned} F_y^{(T_{xy})}\left(X,V_y,V_z\right) = & R\int_{\sqrt{R^2-X^2-V_z^2}}^{V_y}\left(T_y-y\right)y\left(1-\frac{T_z}{\sqrt{R^2-X^2-y^2}}\right)dy \\ = & \frac{1}{2}RT_z\left(R^2-X^2\right)\left(\arcsin\frac{V_y}{\sqrt{R^2-X^2}} + \arcsin\frac{V_z}{\sqrt{R^2-X^2}}\right) \\ & + \frac{1}{2}RT_z\left(2T_y-V_y\right)\sqrt{R^2-X^2-V_y^2} \\ & + \frac{1}{6}R\left(-2V_z^2+3T_zV_z+2R^2-2X^2\right)\sqrt{R^2-X^2-V_z^2} \\ & - \frac{1}{6}R\left(3T_yR^2+2V_y^3-3T_yV_y^2-3T_yV_z^2+6T_yT_zV_z+\frac{6}{4}\pi R^2T_z\right) + R\left(\frac{\pi}{4}T_z+\frac{1}{2}T_y\right)X^2 \end{aligned} \tag{53}$$

and this can be checked by differentiation and evaluation at the limits. Finally, defining

$$\begin{aligned} A &= \frac{1}{6}\left(3T_yR^2+2V_y^3-3T_yV_y^2-3T_yV_z^2+6T_yT_zV_z+\frac{6}{4}\pi R^2T_z\right) \\ B &= \frac{\pi}{4}T_z+\frac{1}{2}T_y \\ C &= -\frac{1}{6}\left(2R^2-2V_z^2+3T_zV_z\right) \end{aligned} \tag{54}$$

we get

$$
\begin{aligned}
G^{(T_{xy})}(X,V_y,V_z) &= \int^X (T_x - x)\, x F_y^{(T_{xy})}(x,V_y,V_z)\,dx \\
&= \frac{1}{2} R T_z \left(T_x R^2 J_1(X;V_y) - R^2 J_2(X;V_y) - T_x J_3(X;V_y) + J_4(X;V_y)\right) \\
&+ \frac{1}{2} R T_z \left(T_x R^2 J_1(X;V_z) - R^2 J_2(X;V_z) - T_x J_3(X;V_z) + J_4(X;V_z)\right) \\
&+ \frac{1}{2} R T_z (2T_y - V_y)\left(T_x I_1\left(X,\sqrt{R^2 - V_y^2}\right) - I_2\left(X,\sqrt{R^2 - V_y^2}\right)\right) \\
&+ R\left(-T_x C I_1\left(X,\sqrt{R^2 - V_z^2}\right) + C I_2\left(X,\sqrt{R^2 - V_z^2}\right) - \frac{1}{3} T_x I_3\left(X,\sqrt{R^2 - V_z^2}\right) + \frac{1}{3} I_4\left(X,\sqrt{R^2 - V_z^2}\right)\right) \\
&- \frac{1}{2} R A T_x X^2 + \frac{1}{3} R A X^3 + \frac{1}{4} R B T_x X^4 - \frac{1}{5} R B X^5
\end{aligned}
\tag{55}
$$

## III. BENCHMARKS

### A. Gaussian profiles: no minimization

Here we document the sensitivity of the calculations to the choice of computational lattice spacing. Table I shows the results as a function of lattice spacing for a LJ potential with cutoff $3\sigma$, using Gaussians with width $\alpha = 230$ (near the minimum) and prefactor 0.995, $k_B T = 0.5\varepsilon$, $\beta\mu = -8.0$ while those for a more localized profile with $\alpha = 1000$ and prefactor 0.95 are given in Table II.

TABLE I. Convergence of the various contributions to the free energy as a function of lattice spacing, $\Delta$, for a Lennard-Jones solid in the Gaussian approximation. The number of points in the calculational cell is $L/\Delta$ and the calculations are for $\alpha = 180\sigma^{-2}$, Gaussian prefactor 0.995, cutoff $r_c = 3\sigma$ and thermodynamic parameters $k_B T = 0.5\varepsilon$, $\beta\mu = -8.0$.

| $\Delta/\sigma$ | $L/\Delta$ | $\beta F_{id}$ | $\beta F_{HS}^{(ex)}$ | $\beta F_{mf}^{(ex)}$ | $\beta\Omega$ |
|---|---|---|---|---|---|
| 0.05 | 32 | 14.20 | 7.79 | −44.62 | 9.21 |
| 0.025 | 64 | 14.20 | 7.25 | −44.62 | 8.67 |
| 0.0125 | 128 | 14.20 | 7.11 | −44.62 | 8.53 |
| 0.00625 | 256 | 14.20 | 7.07 | −44.62 | 8.50 |

TABLE II. Same as Table I for $\alpha = 1000\sigma^{-2}$.

| $\Delta/\sigma$ | $L/\Delta$ | $\beta F_{id}$ | $\beta F_{HS}^{(ex)}$ | $\beta F_{mf}^{(ex)}$ | $\beta\Omega$ |
|---|---|---|---|---|---|
| 0.025 | 64 | 24.44 | 3.90 | -45.68 | 14.50 |
| 0.0125 | 128 | 24.44 | 3.89 | -45.68 | 14.48 |
| 0.00625 | 256 | 24.44 | 3.88 | -45.68 | 14.48 |

### B. Minimized profiles

Finally, we report an example of a system after full minimization with different lattice spacings (see Table III). The Gaussian approximation is seen to be very good with a free energy per unit volume within about 1% of the fully minimized profiles. The free energy and vacancy concentration are already well estimated with a spacing of $0.025\sigma$.

TABLE III. Results of Gaussian approximation and full minimization for a Lennard-Jones solid at constant chemical potential for different lattice spacings. The conditions are the same as given in Table I. The vacancy concentration is from the full mimizations.

| $\Delta/\sigma$ | $L/\Delta$ | $\alpha\sigma^2$ | $\beta\Omega(\text{Gaussian})/V$ | $\beta\Omega(\text{full})/V$ | $C_{vac} = \frac{4-N}{L^3}$ |
|---|---|---|---|---|---|
| 0.05 | 32 | 171.14 | 2.24 | 2.22 | $1.3 \times 10^{-3}$ |
| 0.025 | 64 | 179.01 | 2.11 | 2.08 | $5.9 \times 10^{-4}$ |
| 0.0125 | 128 | 180.41 | 2.08 | 2.05 | $4.9 \times 10^{-4}$ |

## IV. THE FIRE ALGORITHM

The FIRE algorithm is a kind of gradient descent with inertia which means that there is a fictitious velocity for each degree of freedom and a fictitious time variable. Our implementation of the FIRE 2.0 algorithm mostly follows that given in Ref. 1 with the following parameters (using the notation of the reference):

TABLE IV. Parameters used in the FIRE algorithm (variable names following Ref.[1]).

| **Parameter** | **Value** |
|---|---|
| $\Delta t_{\text{start}}$ | 0.1 |
| $\Delta t_{\text{max}}$ | 1.0 |
| $\alpha_{\text{start}}$ | 0.01 |
| $f_\alpha$ | 0.99 |
| $N_{\text{delay}}$ | 5 |
| $N_{\text{max}}$ | 5 |
| $N_{P\leq 0,\text{max}}$ | 20 |
| $f_{\text{inc}}$ | 1.1 |
| $f_{\text{dec}}$ | 0.5 |
| $f_{\text{bak}}$ | 1.1 |

One minor difference in our implementation is that in the case of stopping uphill motion, we reduce the velocities by a factor of 10 rather than setting them to zero. A more substantial customization has to do with backtracking. The FMT part of the free energy functional diverges if the local packing fraction, $\eta(\mathbf{r})$ is equal to or greater than one (a feature, not a bug). Sometimes, the minimization algorithm produces a density which exceeds this threshold and in this case we backtrack: the density and the velocity field are reset to their last valid values and the time step is reduced by a factor of 2. Sometimes, multiple backtracks are necessary before a valid density is field is achieved. Whenever backtracking occurs, the velocities are reduced by a factor of 2 and the maximum timestep is reduced by a factor of 0.8.

We have experimented with different convergence criteria including the root-mean-square force (the force for density degree of freedom $\rho_I$ is $\partial\Lambda[\rho]/\partial\rho_I$), the maximum of the force and the rate of change of the free energy as a function of the fictitious time variable used in the FIRE algorithm. (In the latter case, we use the value of $d\Lambda[\rho]/dt$ exponentially smoothed with smoothing parameter 0.1.) Our minimizations use thresholds of $10^{-9}$ for the rms force, $10^{-10}$ for the maximal force and $10^{-10}$ for the rate of change of the free energy. Our experience is that these criteria are mutually consistent and it is a matter of taste which is used.

[1] Julien Guénolé, Wolfram G. Nöhring, Aviral Vaid, Frédéric Houllé, Zhuocheng Xie, Aruna Prakash, and Erik Bitzek, "Assessment and optimization of the fast inertial relaxation engine (fire) for energy minimization in atomistic simulations and its implementation in lammps," Computational Materials Science **175**, 109584 (2020).
